# Supplementary material for: Cooperative Artificial Intelligence
Source: arXiv:2202.09859 source file (2022-02-20)
Supplement: Supplementary file 1 [file Appendices.tex]

\addcontentsline{toc}{chapter}{Appendices}

% The \appendix command resets the chapter counter, and changes the chapter numbering scheme to capital letters.
%\chapter{Appendices}
\appendix
\chapter{An Appendix About Stuff}
\label{appendixlabel1}
(stuff)

\chapter{Another Appendix About Things}
\label{appendixlabel2}
(things)

\chapter{Colophon}
\label{appendixlabel3}
\textit{This is a description of the tools you used to make your thesis. It helps people make future documents, reminds you, and looks good.}

\textit{(example)} This document was set in the Times Roman typeface using \LaTeX\ and Bib\TeX , composed with a text editor. 
 % description of document, e.g. type faces, TeX used, TeXmaker, packages and things used for figures. Like a computational details section.
% e.g. http://tex.stackexchange.com/questions/63468/what-is-best-way-to-mention-that-a-document-has-been-typeset-with-tex#63503

% Side note:
%http://tex.stackexchange.com/questions/1319/showcase-of-beautiful-typography-done-in-tex-friends
